# Supplementary material for: Looking through the mind's eye via multimodal encoder-decoder networks
Source: arXiv:2410.00047 source file (2024-09-27)
Supplement: Supplementary file 1 [file appendix.tex]

\appendix 
\section{Technical details}

% \subsection{Training}
% \label{sub_section: training}
% Utilizing a common encoder network $g(\cdot|\phi)$, our objective is to align fMRI, Video, and Text prompt representations corresponding to identical emotion classes. Inspired by the recent advancements in meta-learning, we define a task $T$ as a distribution over various combinations of emotion class labels $C$. Specifically, a sampled label set $C$ from task $T$ (expressed as $C \sim T$) typically includes 4 to 20 examples per prompt.

% For the BrainFlux model's encoder $g(\cdot|\phi)$, gradient computation and updating occur during an "episode" initiated by selecting a label set $C$ from task $T$. For example, $C$ might comprise the label set {Yale, Awe}. Utilizing $C$, we then draw samples from fMRI support sets $S_{f}$, video sets $S_{v}$, and text sets $S_{t}$, where each set contains labeled instances of Yale and Awe. More precisely, our training objective is as follows
% \begin{equation} \nonumber
%     \begin{aligned}
%         \phi = \arg \max_{\phi} \mathbb{E}_{C \sim T} \Biggl[ \mathbb{E}_{\{S_{f} \sim C\}, \{S_{v} \sim C\}, \{S_{t} \sim C\}} \Biggl[ \sum_{\substack{(x_\text{f}, y) \in S_\text{f} \\ (x_\text{v}, y) \in S_\text{v} \\ (x_t, y) \in S_t}}  \log P_{\phi} (y|x_\text{f}, x_\text{v}, x_t)\Biggl] \Biggl].
%     \end{aligned}
% \end{equation}

% \newpage
\subsection{Video Reconstruction}
\label{sub_section: video_training}
The initial encoder, denoted as $g_\text{v}(\cdot|\phi_\text{v})$, and decoder, denoted as $f_\text{v}(\cdot|\theta_\text{v})$, form a video-specific model architecture designed to learn representations by reconstructing video frames, thereby facilitating the learning of embeddings.
\begin{align}
    \frac{1}{|S_\text{v}|} \sum_{ \mathbf{x}_{\text{v}, i}\in S_\text{v}} ||\mathbf{x}_{\text{v}, i}- f_\text{v}(g_\text{v}(\mathbf{x}_{\text{v}, i}|\phi_\text{v}) | \theta_\text{v}) ||^2, 
\end{align}
where $\mathbf{x}_{\text{v}, i}$ is a frame of a video $S_\text{v}$. Beside, $\theta_\text{v}$ and $\phi_\text{v}$ are the parameters of the $f_\text{v}$ and $g_\text{v}$, respectively.

\subsection{fMRI of Video Prompt Reconstruction}
Equipped with the video reconstruction autoencoder, we proceed to construct an fMRI encoder, \(g_{\text{f}}(\cdot|\phi_{\text{f}})\), and decoder, \(f_{\text{f}}(\cdot|\theta_{\text{f}})\), architecture specifically tailored to learn the representations of brain recordings stimulated by video. With these dual encoder-decoder architectures for video and fMRI, we now build a bridge to create a learning module that translates the fMRI encoder's output into the video encoder's input. To this end, we employ a lightweight mapping function, \(\text{MAP}_{\text{f} \rightarrow \text{v}}(\cdot) = q(\cdot | W_{\text{q}})\), that aims at point-to-point matching fMRI embeddings with their corresponding video frames to which the brain has been exposed. Given these elements, the overall loss function for training the fMRI encoder-decoder and refining the encoder for both fMRI and video would be as follows:

\begin{align}
    \frac{1}{|S_\text{f}|} \sum_{ \mathbf{x}_{\text{f}, i}\in S_\text{f}} ||\mathbf{x}_{\text{f}, i}- f_\text{f}(g_\text{f}(\mathbf{x}_{\text{f}, i}|\phi_\text{f}) | \theta_\text{f}) ||^2  + 
    \frac{1}{|S_\text{f}|} 
    \sum_{\substack{(\textbf{x}_{\text{v}, i}) \in S_\text{v} \\ (\textbf{x}_{\text{f}, i}) \in S_\text{f} }} \|  g_\text{v}(\mathbf{x}_{\text{v}, i}|\phi_\text{v}) -     
    \text{MAP}_{\text{f} \rightarrow \text{v}}(g_\text{f}(\mathbf{x}_{\text{f}, i}|\phi_\text{f})\|^2, 
\end{align}
where $\mathbf{x}_{\text{f}, i}$ is a frame of an fMRI recording while the brain has been stimulated by video $S_\text{f}$, and $|S_\text{f}| = |S_\text{v}|$. Beside, $\theta_\text{f}$ and $\phi_\text{f}$ are the parameters of the $f_\text{f}$ and $g_\text{f}$, respectively.

\subsection{fMRI of Emotion Prompt Reconstruction}

After developing architectures for video and video-prompted fMRI encoder-decoder, our next step is to train an emotion-prompted fMRI encoder, \(g_{\text{e}}(\cdot|\theta_{\text{e}})\), and decoder, \(f_{\text{e}}(\cdot|\phi_{\text{e}})\). It's important to note that emotion-prompted brain recordings lack a direct point-to-point correlation with the video content. Thus, we aim to align the emotion-based distribution with that of the distribution derived from visually and emotionally stimulated brain recordings. Despite science videos or visual content possessing emotional labels, we undertake the task of emotion-based distribution-to-distribution matching. Our strategy involves guiding the embeddings of emotionally stimulated brain recordings closer to those from visually stimulated recordings. Mathematically, we begin by calculating the prototype for the \(k\)-th class \(C\) in the visually stimulated fMRI context, denoted by \(\mathbf{p}_\text{v}^k\):

\begin{align} 
    \mathbf{p}_\text{f}^k &= \frac{1}{S^k_\text{f}} \sum_{(\mathbf{x}_\text{f}^i, {y}^i) \in S^k_\text{f}} g_{\text{f}}(\mathbf{x}_\text{f}^i | \phi_\text{f}),
\end{align}
where \(\mathbf{p}_\text{f}^k\) represents the centroid of the fMRI recordings for subjects watching an emotional video from the \(k\)-th class. We subsequently apply an MLP-based mapping function, \(\text{MAP}_{\text{e} \rightarrow \text{f}}(\cdot) = h(\cdot|W_{\text{h}})\), to align emotionally stimulated fMRI recordings with visually stimulated fMRI recordings that share the same emotion label. To achieve this, we use a distance function \(d(\cdot, \cdot)\). Specifically, we define a cross-entropy loss function to perform emotion-based distribution matching based on the following softmax function:
\begin{align}
    P_{\phi} (y=k | \mathbf{p}_\text{f}^k) = 
    \frac{\exp\big(-d \big(\text{MAP}_{\text{e} \rightarrow \text{f}}(g_{\text{e}}(\mathbf{x}^i_{\text{e}}|\phi_\text{e})), \mathbf{p}_\text{f}^k\big)\big)}
    {\sum_{k'}\exp\big(-d \big(\text{MAP}_{\text{e} \rightarrow \text{f}}(g_{\text{e}}(\mathbf{x}^i_{\text{e}}|\phi_\text{e})), \mathbf{p}_\text{f}^{k'}\big)\big)}, 
\end{align}
The learning process progresses by minimizing the negative log-probability \(J(\phi) = -\log P_{\phi}(y=k | \mathbf{x})\) of the correct class \(k\) through Stochastic Gradient Descent (SGD). Moreover, we employed a mean-squared loss function for representation learning of the emotionally stimulated brain recordings by both the encoder and decoder.
